# Supplementary material for: Improving Code Review with GitHub Issue Tracking
Source: arXiv:2210.04434 source file (2022-10-10)
Supplement: Supplementary file 1 [file appendix.tex]

\begin{algorithm}
\label{alg:Alg1}
\SetAlgoLined
\KwData{The initial set, \textit{\textbf{IssuesSet}}, that includes all Issue events of the repository \textit{\textbf{R}} that are opened within the \textit{\textbf{initial assessment period}} = $x$ days.}
\KwResult{Set of regularly opened Issues.}
let \textit{ICD} = []\;
\For{(each \textbf{issue} in \textbf{IssuesSet})}{
\textit{ICD}.append(\textbf{\textit{issues}}.creationDate())\;
}
\textit{D} = []\;
\For{(each adjacent pare ($d_1$, $d_2$) in ICD)}{
let \textit{timeDistance} = ($d_2$ - $d_1$).days()\;
\textit{D}.append(\textit{timeDistance})\;
}
let \textit{IDM} = \textit{D}.median()\;
let \textit{waitTime} = \textit{IDM}\;
\While{True}{
\While{the elapsed time since the last Issue of IssuesSet $<$ waitTime}{
\If{a new Issue is opened}{
\textit{IssueSet}.append(\textit{new Issue})\;
let \textit{d} = time distance between the last two Issues of \textit{IssuesSet}\;
\textit{D}.append(\textit{d})\;
\textit{IDM} = \textit{D}.median()\;
\textit{waitTime} = \textit{IDM}\;
}
}
Send \textbf{\textit{NewIssueNotification}}(\textit{R})\;
\textit{waitTime} = \textit{waitTime} + \textit{IDM}\;
}

\caption{New Issue Notifier (NIN) where \textit{ICD} is the set of Issues Creation Date, \textit{D} is the set of temporal distances between Issues, and \textit{IDM} is the Issue Distances median. }
\end{algorithm}
